# Supplementary material for: Gastric-X: A Multimodal Multi-Phase Benchmark Dataset for Advancing Vision-Language Models in Gastric Cancer Analysis
Source: arXiv:2603.19516 source file (2026-03-26)
Supplement: Supplementary file 1 [file supp_tables_plain.tex]

% Auto-generated plain table version
\begin{table*}[t]
\centering
\begin{tabular}{l p{6cm} l p{6cm}}
\toprule
Item & Description & Item & Description \\
\midrule
Hospital ID (De-identified) & Anonymized hospitalization identifier & Patient Name (De-identified) & Anonymized patient name code \\
Sex & Biological sex & Age (De-identified) & Age at admission (de-identified) \\
Bed Number (De-identified) & Anonymized bed assignment & Surgery Date (De-identified) & Date of surgery (de-identified) \\
Imaging ID & CT imaging identifier & CT Description & Radiology morphological description \\
CBC: Test Date & Date of CBC test & CBC: White Blood Cell Count & White blood cell count (×10^9/L) \\
CBC: Neutrophil Count & Absolute neutrophil count (×10^9/L) & CBC: Neutrophil Ratio & Neutrophil percentage (\%) \\
CBC: Lymphocyte Count & Absolute lymphocyte count (×10^9/L) & CBC: Lymphocyte Ratio & Lymphocyte percentage (\%) \\
CBC: Hemoglobin & Hemoglobin concentration (g/L) & CBC: Platelet Count & Platelet count (×10^9/L) \\
Biochemistry: Test Date & Date of biochemistry test & Biochemistry: Fasting Glucose & Fasting plasma glucose (mmol/L) \\
Biochemistry: Prealbumin & Serum prealbumin (mg/L) & Biochemistry: ALT & Alanine aminotransferase (U/L) \\
Biochemistry: AST & Aspartate aminotransferase (U/L) & Biochemistry: Total Protein & Total serum protein (g/L) \\
Biochemistry: Albumin & Serum albumin (g/L) & Biochemistry: Total Bilirubin & Total bilirubin (µmol/L) \\
Biochemistry: Direct Bilirubin & Direct bilirubin (µmol/L) & Biochemistry: Creatinine & Serum creatinine (µmol/L) \\
Biochemistry: Urea (BUN) & Blood urea nitrogen (mmol/L) & Tumor Markers: Test Date & Date of tumor marker test \\
Tumor Markers: AFP & Alpha-fetoprotein (AFP) & Tumor Markers: CEA & Carcinoembryonic antigen (CEA) \\
Tumor Markers: CA125 & Cancer antigen 125 (CA125) & Tumor Markers: CA724 & Cancer antigen 724 (CA724) \\
Tumor Markers: CA199 & Cancer antigen 19-9 (CA19-9) & Past Medical History: Conditions (Not Used) & Past medical conditions (record retained but not used in experiments) \\
Surgical/Trauma History (Not Used) & Prior surgical or trauma history (retained but not used) & Hospital ID (De-identified) & Anonymized hospitalization identifier \\
Patient Name (De-identified) & Anonymized patient name code & Sex & Biological sex \\
年龄 & Clinical variable & 床号 & Clinical variable \\
手术日期 & Clinical variable & Resection Range & Extent of resection \\
Gastrointestinal Reconstruction & Type of reconstruction after resection & Occupation & Patient occupation (anonymized) \\
Education Level & Highest educational attainment & Marital Status & Marital status \\
Ethnicity & Ethnic group & Admission Method & Mode of hospital admission \\
Insurance Status & Medical insurance coverage & ID Number (De-identified) & Identification document number (anonymized) \\
Contact Number (De-identified) & Contact phone (anonymized) & Surgery Admission Date (De-identified) & Date of admission for surgery (de-identified) \\
Surgery Discharge Date (De-identified) & Date of discharge after surgery (de-identified) & Surgery Hospitalization Cost & Total cost for surgical hospitalization (local currency) \\
Admission Temperature & Body temperature at admission (°C) & Admission Pulse & Pulse rate at admission (beats/min) \\
Admission Respiration & Respiratory rate at admission (breaths/min) & Admission Systolic Pressure & Systolic blood pressure at admission (mmHg) \\
Admission Diastolic Pressure & Diastolic blood pressure at admission (mmHg) & Height & Height (cm) \\
Weight & Weight (kg) & BMI & Body mass index (kg/m^2) \\
General Condition & Clinical performance status (qualitative) & Weight Loss & Recent unintended weight loss \\
Reduced Food Intake & Decrease in oral intake & Smoking Status & Current/former/never smoker \\
Drinking Status & Alcohol consumption status & Endoscopy Date (De-identified) & Date of gastroscopy (de-identified) \\
Endoscopy Tumor Location & Tumor location observed in endoscopy & Endoscopy Tumor Size & Tumor size measured in endoscopy (cm) \\
Endoscopy Gross Type & Endoscopic macroscopic classification & Endoscopy Biopsy Pathology & Biopsy-based pathological diagnosis \\
Endoscopy Appearance & Endoscopic visual findings & Chief Surgeon (De-identified) & Primary operating surgeon (anonymized) \\
First Assistant (De-identified) & Primary assistant surgeon (anonymized) & Surgery Nature & Elective/emergency \\
Surgery Mode & Open or minimally invasive & Lymphadenectomy Extent & Extent of lymph node dissection \\
Combined Resections & Concurrent organ resections & Surgery Start Time (De-identified) & Operation start time (de-identified) \\
Surgery End Time (De-identified) & Operation end time (de-identified) & Surgery Duration & Total operative time (minutes) \\
Intraoperative Blood Loss & Estimated blood loss (mL) & Transfused Red Blood Cells & Units of RBC transfused \\
Transfused Plasma & Volume of plasma transfused & Intraoperative Transfusion & Any transfusion during surgery \\
Residual Tumor (Intraoperative) & Macroscopic residual tumor status & Drainage Tube & Presence of drainage tube \\
Additional Procedures & Other intraoperative procedures & Tumor Anatomical Location & Anatomical site of the tumor \\
Tumor Lateral Position & Lateral orientation of tumor & Maximum Tumor Diameter & Maximal tumor diameter (cm) \\
Serosal Invasion & Serosal layer involvement (Y/N) & Gross Tumor Type & Macroscopic tumor classification \\
Linitis Plastica & Presence of linitis plastica (Y/N) & Perigastric Lymph Nodes & Status of perigastric nodes \\
Liver Metastasis & Presence of hepatic metastases (Y/N) & Adjacent Organ Invasion & Invasion of neighboring organs (Y/N) \\
Peritoneal Seeding & Peritoneal metastasis (Y/N) & Ascites & Presence of ascites (Y/N) \\
Pathology ID (De-identified) & Anonymized pathology specimen identifier & Tumor Size - Long Axis & Pathology long-axis measurement (cm) \\
Tumor Size - Short Axis & Pathology short-axis measurement (cm) & Tumor Size - Height & Tumor height (cm) \\
Primary Histologic Type & Main histological subtype & Histologic Grade & Tumor differentiation grade \\
Additional Histologic Type & Other histologic components & Distance to Proximal Margin & Distance from tumor to proximal margin (cm) \\
Distance to Distal Margin & Distance from tumor to distal margin (cm) & Specimen Proximal Margin & Proximal margin status (specimen) \\
Specimen Distal Margin & Distal margin status (specimen) & Perineural Invasion & Perineural invasion (Y/N) \\
Vascular Cancer Thrombus & Vascular invasion / intravascular tumor thrombus (Y/N) & Greater Omentum Invasion & Invasion of greater omentum (Y/N) \\
Lesser Omentum Invasion & Invasion of lesser omentum (Y/N) & Greater Omentum Metastasis & Metastasis to greater omentum (Y/N) \\
Lesser Omentum Metastasis & Metastasis to lesser omentum (Y/N) & Multifocal Tumors & Presence of multiple tumor foci (Y/N) \\
Positive Lymph Nodes & Number of positive lymph nodes & Dissected Lymph Nodes & Total number of dissected lymph nodes \\
T Stage & Pathological T category & N Stage & Pathological N category \\
M Stage & Pathological M category & Overall Stage & Overall pathologic stage \\
Surgical Radicality & R0/R1/R2 resection status & Group 1 Positive & Group 1 positive node count \\
Group 1 Dissected & Group 1 dissected count & Group 2 Positive & Group 2 positive node count \\
Group 2 Dissected & Group 2 dissected count & Group 3 Positive & Group 3 positive node count \\
Group 3 Dissected & Group 3 dissected count & Group 4 Positive & Group 4 positive node count \\
Group 4 Dissected & Group 4 dissected count & Group 5 Positive & Group 5 positive node count \\
Group 5 Dissected & Group 5 dissected count & Group 6 Positive & Group 6 positive node count \\
Group 6 Dissected & Group 6 dissected count & Groups 7/8/9 Positive & Groups 7/8/9 positive node count \\
Groups 7/8/9 Dissected & Groups 7/8/9 dissected count & Greater Curvature Positive & Positive nodes on greater curvature \\
Greater Curvature Dissected & Dissected nodes on greater curvature & Lesser Curvature Positive & Positive nodes on lesser curvature \\
Lesser Curvature Dissected & Dissected nodes on lesser curvature & Other Stations Positive & Other nodal station positive count \\
Other Stations Dissected & Other nodal station dissected count & Ki-67 & Proliferation index (IHC) \\
HER2 Status & HER2 receptor status (IHC) & CLDN Status & Claudin expression status \\
MLH1 & MLH1 expression (IHC) & PMS2 & PMS2 expression (IHC) \\
MSH2 & MSH2 expression (IHC) & MSH6 & MSH6 expression (IHC) \\
EBER & EBV-encoded RNA by ISH & PD-L1 Score & PD-L1 immunohistochemistry score \\
MMR Status & Mismatch repair status & PD-L1 Status & PD-L1 categorical status \\
Complication Severity & Clavien–Dindo grade & Secondary Surgery & Reoperation required (Y/N) \\
Complication Occurrence & Any postoperative complication (Y/N) & Complication Present & Whether complication occurred (Y/N) \\
Severe Complication Occurrence & Severe complication (Y/N) & Total Hospital Stay (Days) & Total days hospitalized for surgery \\
Postoperative Stay (Days) & Days hospitalized after surgery & Preoperative Transfusion & Any transfusion before surgery \\
Postoperative Transfusion & Any transfusion after surgery & Postoperative Fever & Fever after surgery (Y/N) \\
Fever Days & Number of days with postoperative fever & Complication Category & Type/category of complication \\
Intervention & Management or treatment measures & Complication Notes & Additional notes on complications \\
\bottomrule
\end{tabular}
\end{table*}
